# Supplementary material for: Multiple-Play Stochastic Bandits with Shareable Finite-Capacity Arms
Source: arXiv:2206.08776 source file (2022-06-17)
Supplement: Supplementary file 1 [file appendix_simpler_algorithm.tex]

% !TeX root = ../sharing_bandits.tex
\section{Algorithms}\label{app:simple_algo}

\subsection{MP-SE in Algorithm~\ref{alg:mp_se}}\label{appsub:mp_se}

\begin{algorithm}[htb]
	\caption{Multiple-Play Successive Elimination (MP-SE)}
	\label{alg:mp_se}
	{\bfseries Input:} Arm set $[K]$, plays $N$, time horizon $T$, and parameters $\gamma\in [1,\infty)$.\\
	{\bfseries Initial:} $t,\tau_t \gets 1,\, \mathcal{S}\gets [K],\, \hat{\bm{\mu}}_t\gets\bm{0}\in \mathbb{R}^K.$
	\begin{algorithmic}[1]
		\While{$t\le T$}
		\State{Sort $\{\hat{\mu}_{k,t}, k \in \mathcal{S}\}$ via a mapping $\sigma$, such that $\hat{\mu}_{\sigma(k),t}$ is the $k$th largest among them.}
		\If{$N < \abs{\mathcal{S}}$}\Comment{Use $N$ to replace $\hat{L}_t$.}
		\State{\textsc{Elimination}($\mathcal{S}, \hat{\bm{\mu}}_t, \sigma(\cdot),\gamma,T$).}
		\State{\scshape Individual Exploration($\mathcal{S}, \hat{\bm{\mu}}_t, \tau_t, t$).}
		% \For {$k\in \mathcal{S}$ }
		% \If {$\hat{\mu}_{k,t} \le \hat{\mu}_{\sigma(N),t} - \gamma U(\tau_t, T)$}
		% \State $\mathcal{S}\gets \mathcal{S}\setminus\{k\}.$ \Comment{Elimination}
		% \EndIf
		% \EndFor
		% \State{Individually explore $\mathcal{S}$ and update $\hat{\bm{\mu}}_t.$ \Comment{Proc.~\ref{alg:ie}}}
		% % }
		% \State{
		% 	$\tau_t \gets \tau_t + 1$, $t\gets t+\ceil{\abs{\mathcal{S}}/N}.$
		% }
		\ElsIf{$N = \abs{\mathcal{S}}$}
		\State{\scshape Exploitation($\mathcal{S},\hat{\bm{m}}_t^l,\hat{\bm{\mu}}_t,\hat{L}_t,\sigma(\cdot),\tau_t, t$).}
		\EndIf
		\EndWhile
	\end{algorithmic}
\end{algorithm}

\subsection{MP-SA-SA-KC in Algorithm~\ref{alg:mp_se_sa_kc}}\label{appsub:mp_se_ksa}

\begin{algorithm}[htb]
	\caption{MP-SE-SA-KC}
	\label{alg:mp_se_sa_kc}
	{\bfseries Input:} Arm set $[K]$, plays $N$, time horizon $T$, sharing capacity $\bm{m}$ and parameters $\gamma\in [1,\infty)$.\\
	{\bfseries Initial:} $t,\tau_t\gets 1,\, \mathcal{S}\gets [K],\, \hat{\bm{\mu}}_t\gets\bm{0}\in \mathbb{R}^K,\,  \hat{L}_t\gets N.$
	\begin{algorithmic}[1]
		\While{$t\le T$}
		\State{Sort $\{\hat{\mu}_{k,t}, k \in \mathcal{S}\}$ via a mapping $\sigma$, such that $\hat{\mu}_{\sigma(k),t}$ is the $k$th largest among them.}
		\State{$\hat{L}_t\gets \argmin_n\left\{n:\sum_{k=1}^n {m}_{\sigma(k),t}\ge N\right\}.$}

		\If{$\hat{L}_t < \abs{\mathcal{S}}$}
		\State{\textsc{Elimination}($\mathcal{S}, \hat{\bm{\mu}}_t, \sigma(\cdot),\gamma,T$).}
		\State{\scshape Individual Exploration($\mathcal{S}, \hat{\bm{\mu}}_t, \tau_t, t$).}
		% }
		% \State{
		% 	$\tau_t \gets \tau_t + 1$, $t\gets t+\ceil{\abs{\mathcal{S}}/N}.$
		% }
		\ElsIf{$\hat{L}_t = \abs{\mathcal{S}}$}
		\State{\scshape Exploitation($\mathcal{S},\hat{\bm{m}}_t^l,\hat{\bm{\mu}}_t,\hat{L}_t,\sigma(\cdot),\tau_t, t$).}
		\EndIf
		% \State $\tau_t\gets \tau_t + 1$
		\EndWhile
	\end{algorithmic}
\end{algorithm}
