# Supplementary material for: Multiple-Play Stochastic Bandits with Shareable Finite-Capacity Arms
Source: arXiv:2206.08776 source file (2022-06-17)
Supplement: Supplementary file 2 [file appendix_simulations.tex]

% !TeX root = ../sharing_bandits.tex

\section{Additional Simulations}

\subsection{Impact of parameters $\gamma$ and $\xi$. } \label{appsub:impact_of_gma_xi}
% ADD an $\xi$ comparison and show its exploration control ability.
Parameters $\gamma$ and $\xi$ can be tuned for better performance in specific bandits environment but simply setting both as $1$ is also valid. Figure~\ref{subfig:gamma_impact} shows that a higher $\gamma$ causes more explorations and thus higher regret.
%  and thus smaller regret variance (e.g., the green line with $\gamma =5$'s variance is negligible).
% , which confronts with the fact that $\gamma=1$ is the more aggressive.
Figure~\ref{subfig:xi_impact} shows that the smaller the $\xi$, the more aggressive in estimating capacities. Specifically, the red line of $\xi=0.01$ in Figure~\ref{subfig:xi_impact} implies that the lack of exploration leads to a linear regret and high variance.
We set $\gamma=1$ and $\xi=0.05$ as default in remaining simulations.

\begin{figure*}[htb]
    \centering
    \subfloat[The impact of parameter $\gamma$ ($\xi=0.05$)\label{subfig:gamma_impact}]{\includegraphics[width=0.71\columnwidth]{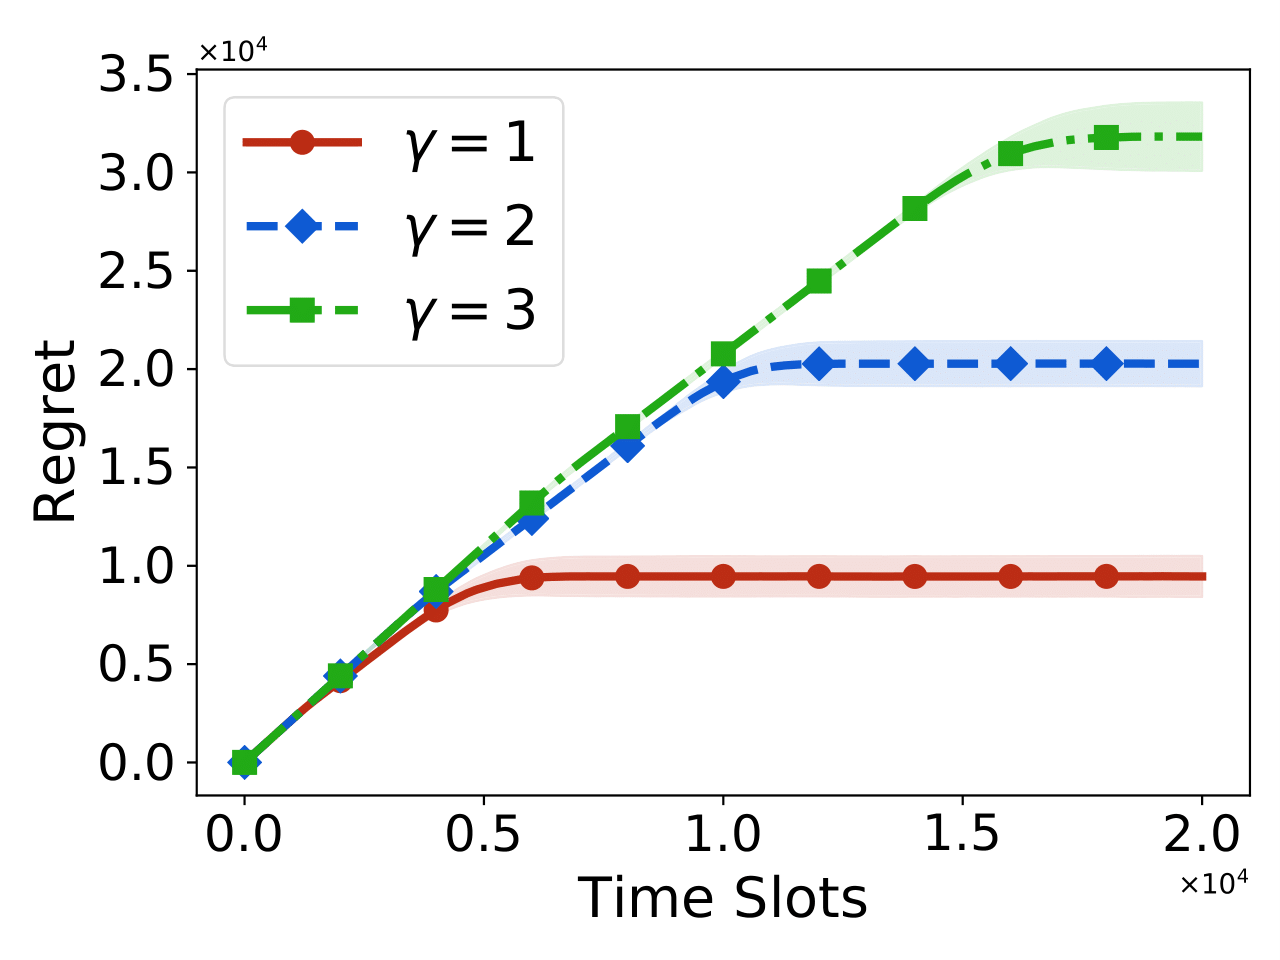}}
    \subfloat[The impact of parameter $\xi$ ($\gamma=1$)\label{subfig:xi_impact}]{\includegraphics[width=0.71\columnwidth]{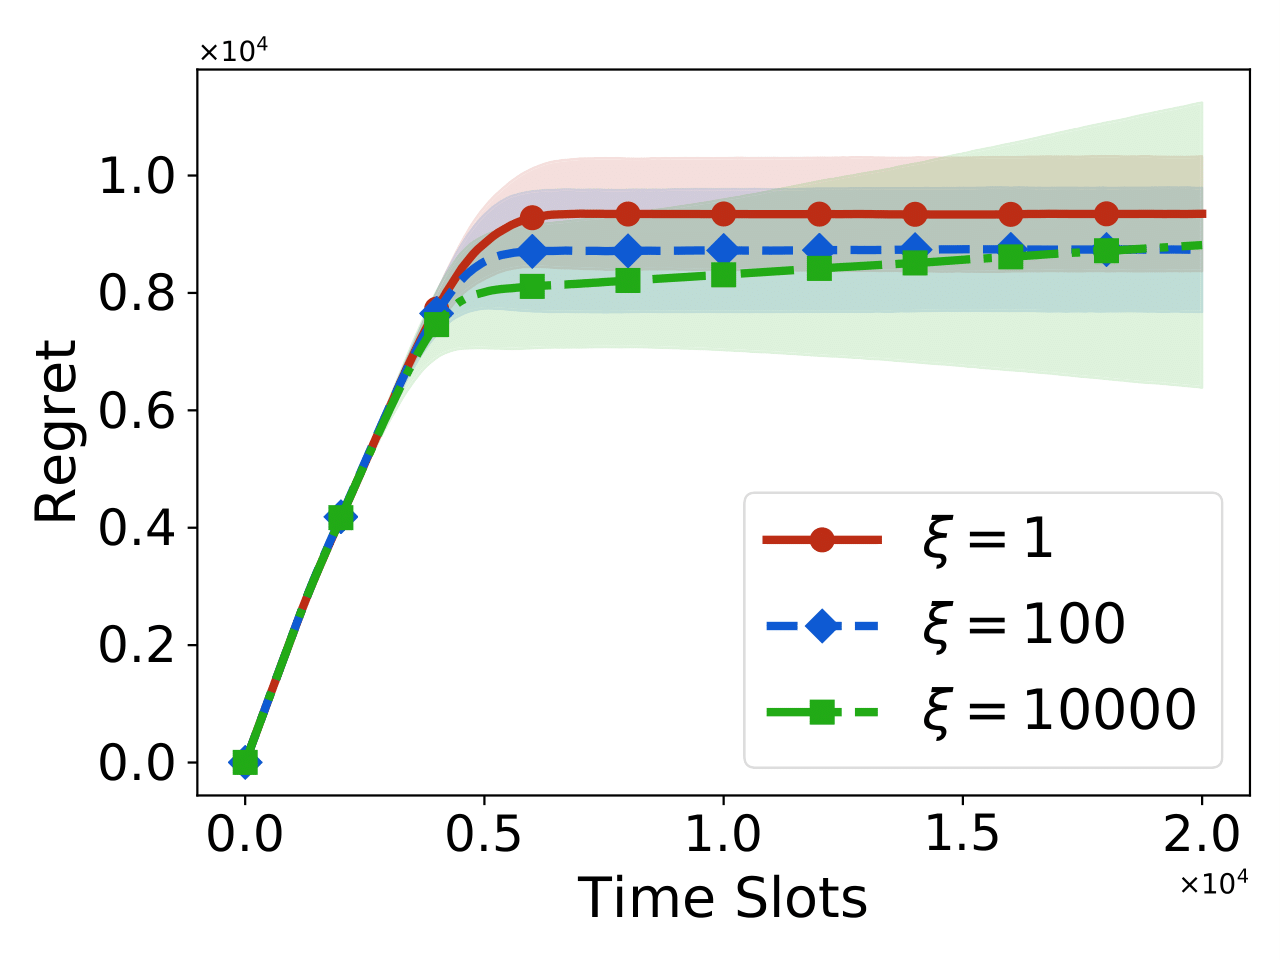}}
    \caption{Numerical Simulations}
    \label{fig:numerical}
\end{figure*}
